# Supplementary material for: Observation of the $B^0_s\!\to D^{*+}D^{*-}$ decay
Source: arXiv:2210.14945 source file (2023-07-17)
Supplement: Supplementary file 1 [file supplementary.tex]

\clearpage

\section{Supplementary material for LHCb-PAPER-2022-023}
\label{sec:Supplementary-App}

This appendix contains supplementary material that will be posted
on the public CDS record but will not appear in the paper.

\subsection{Combined mass fit plot}
\begin{figure}[h]
  \centering
  \includegraphics[width=0.49\textwidth]{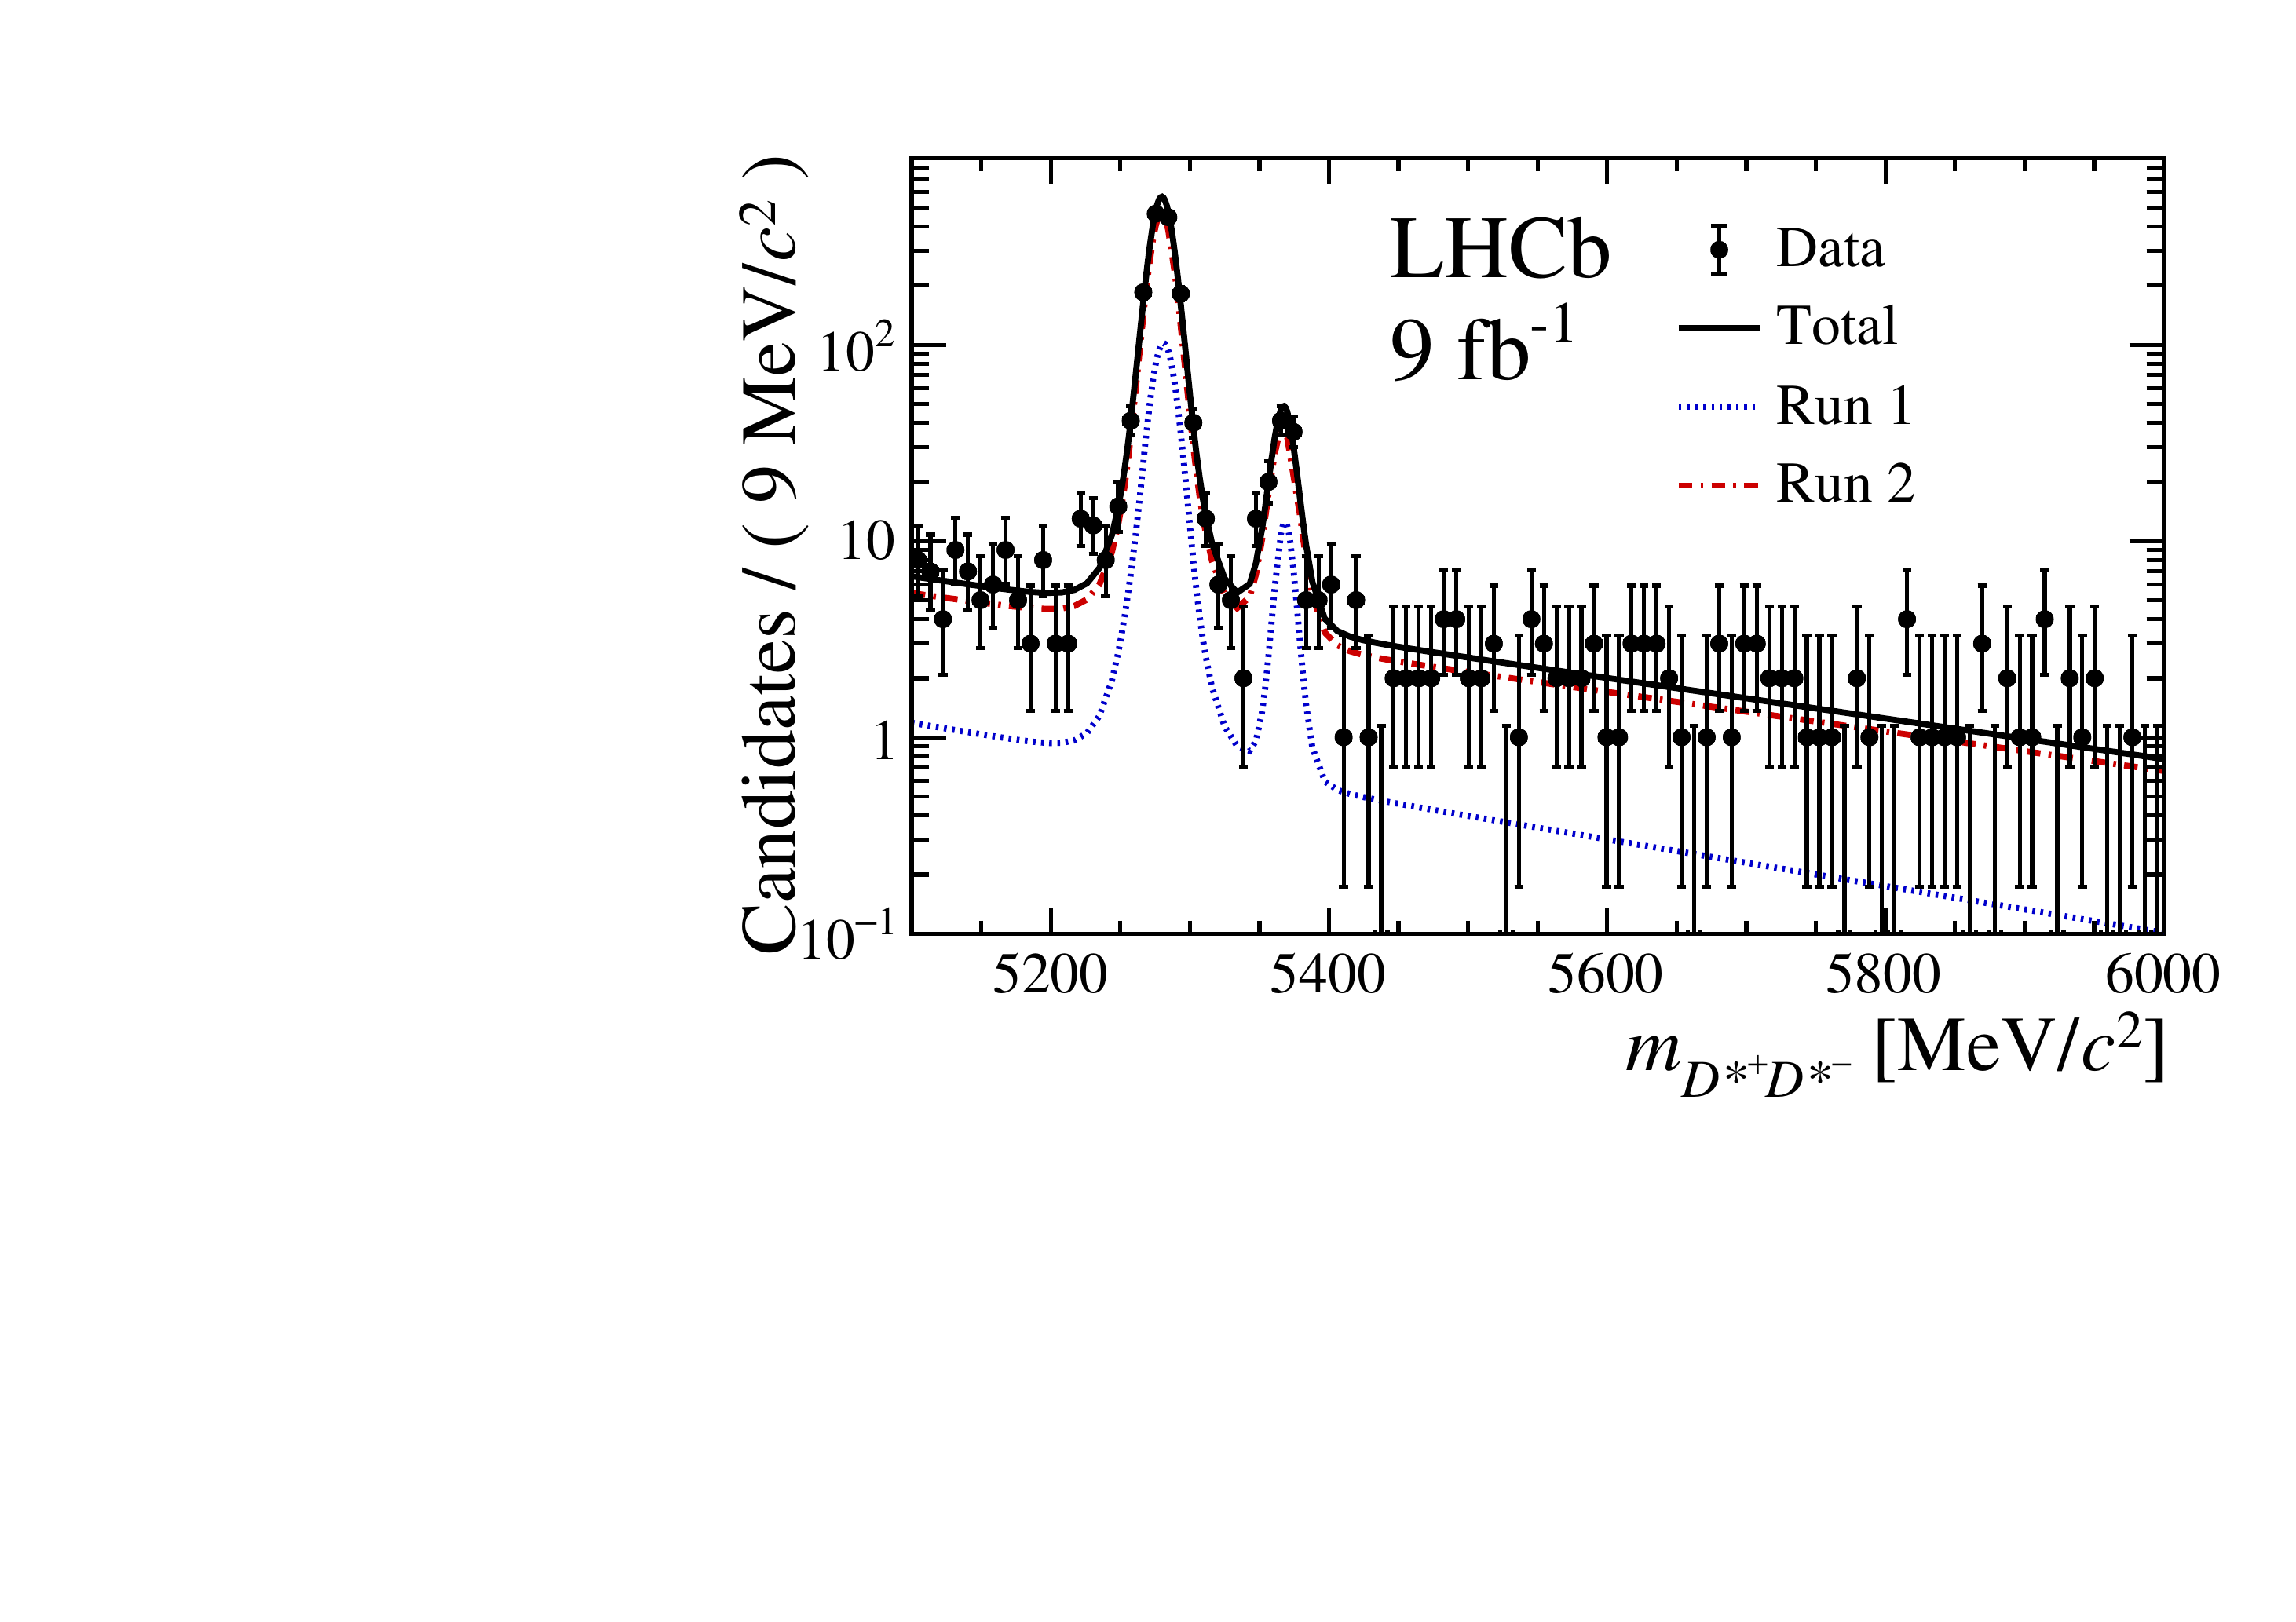}
  \includegraphics[width=0.49\textwidth]{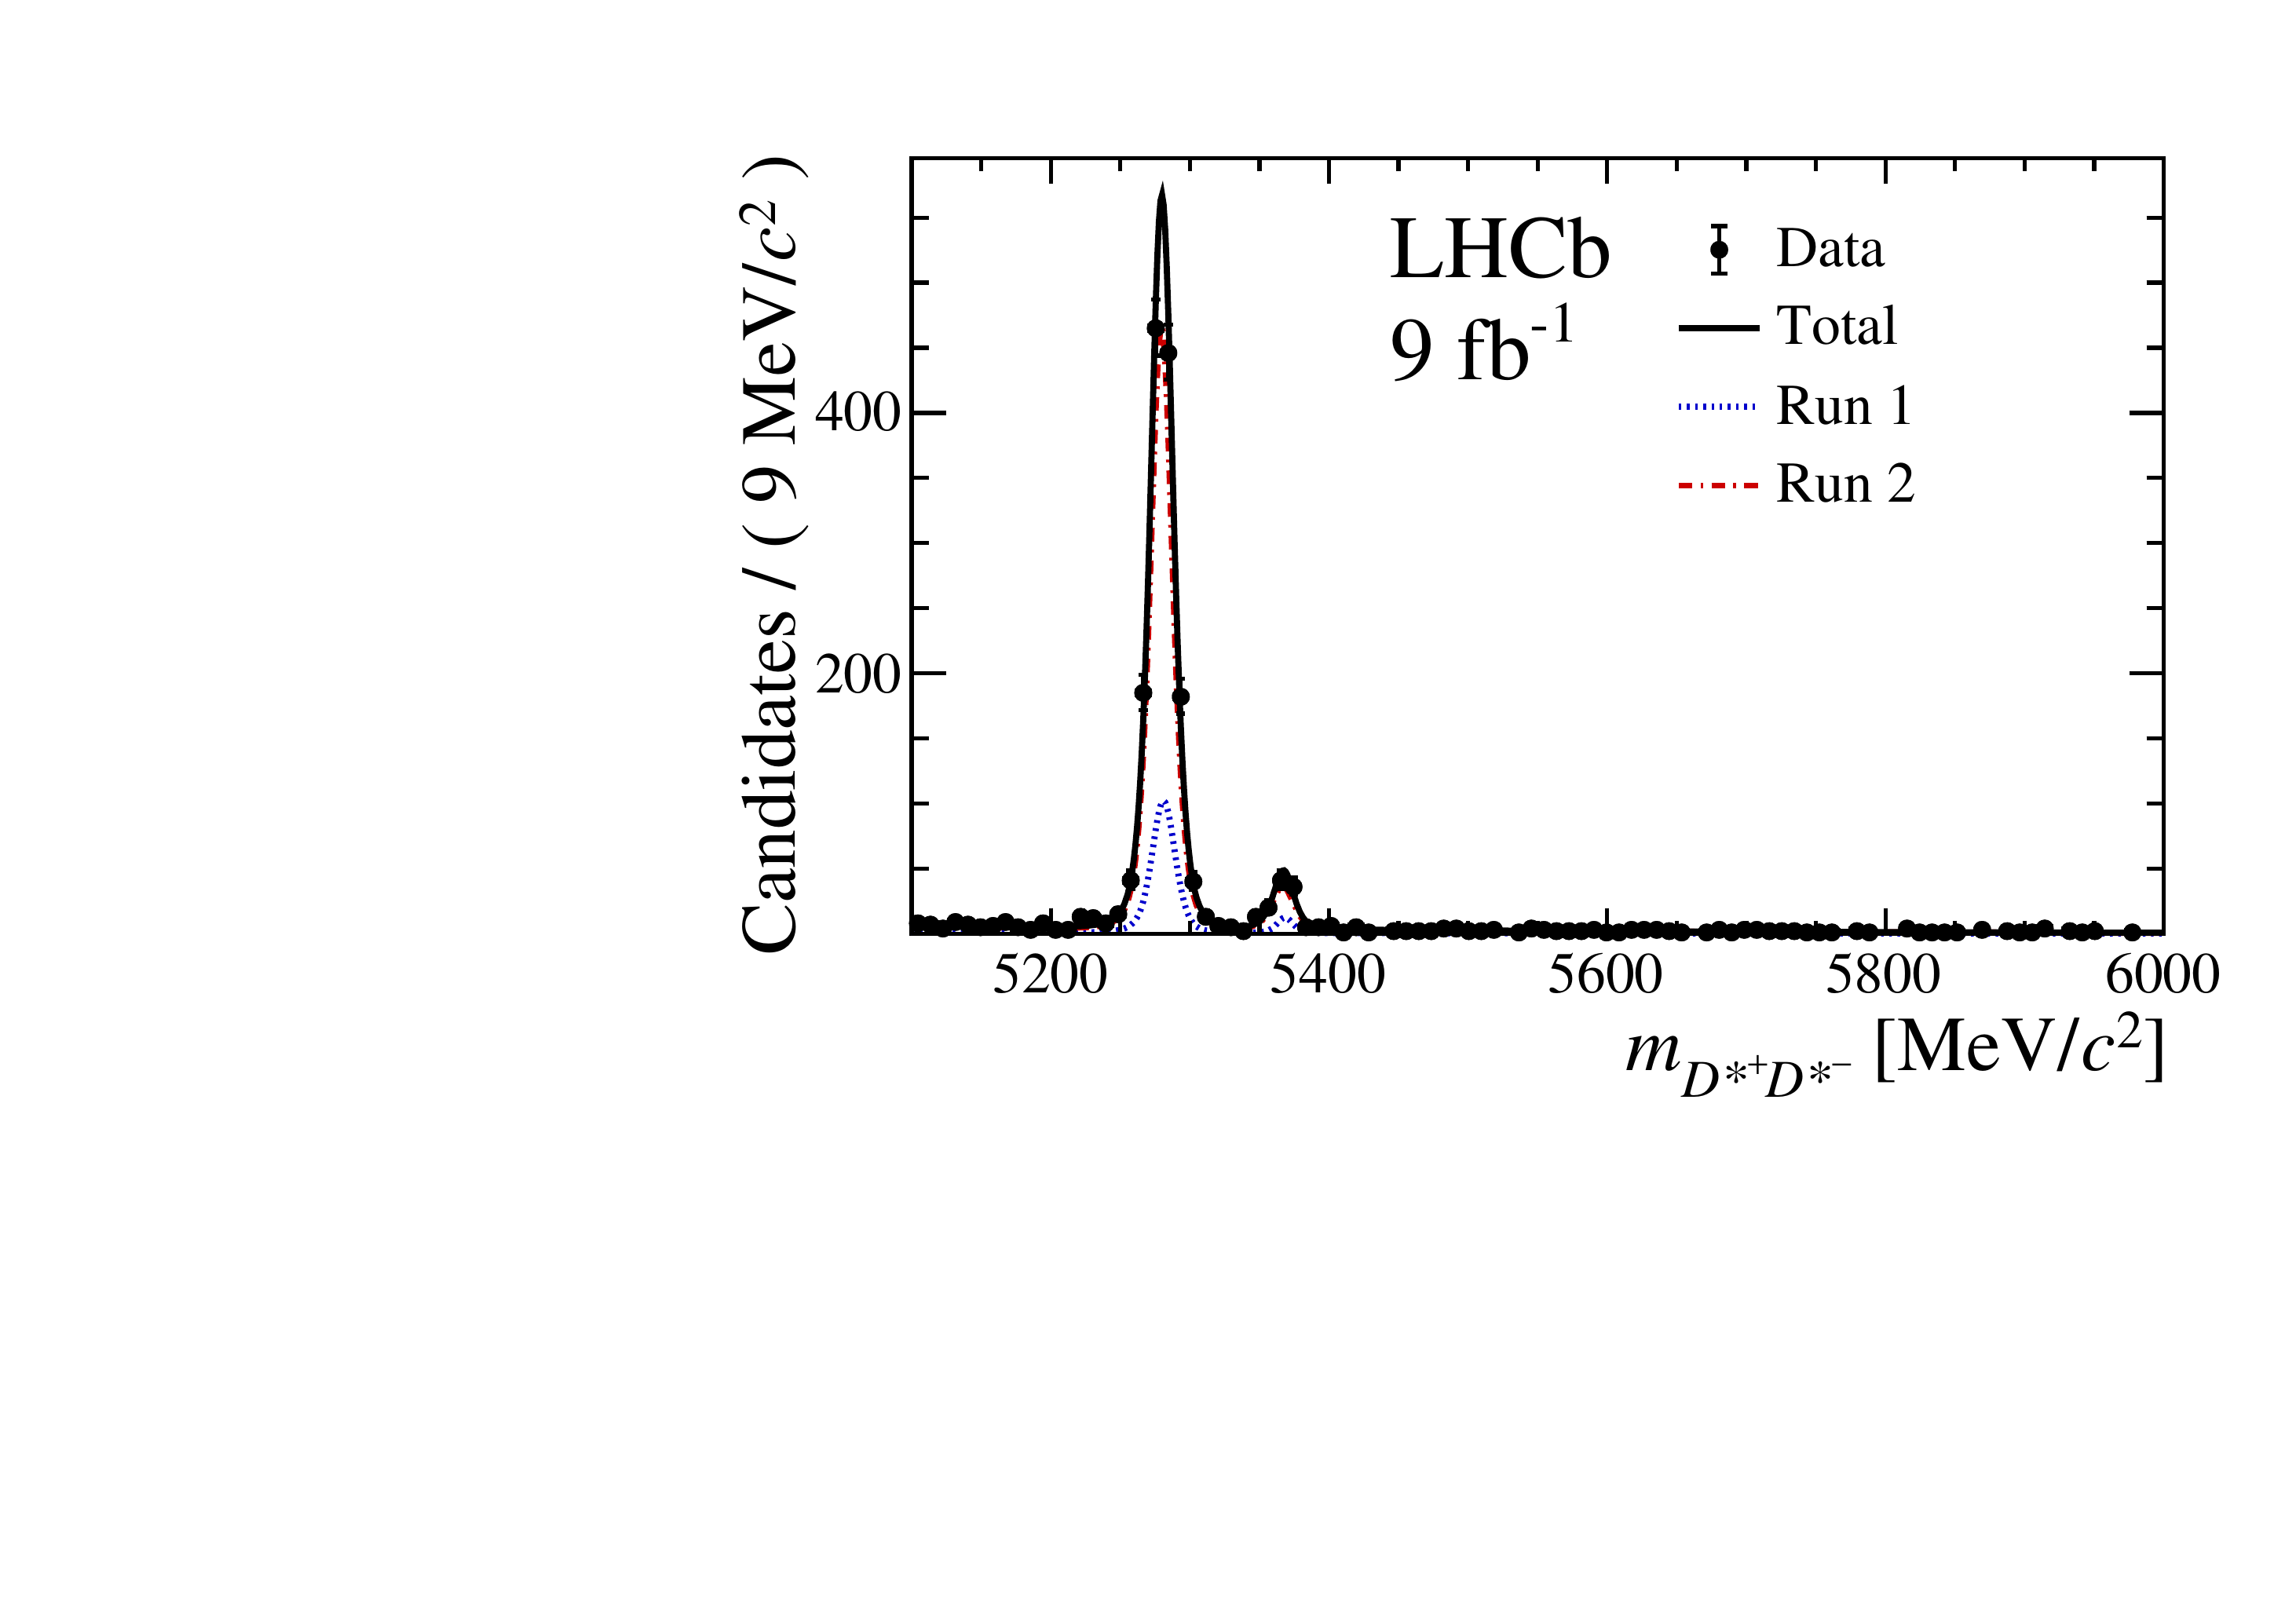}\\
  \caption{Distributions of the \Dstarp\Dstarm mass combining both data-taking periods with (left) 
  logarithmic and (right) linear $y$ axes.
  In addition to the total fit result (solid black), each of the individual components are shown: the (dotted blue) Run 1 and the (dash-dotted red) Run 2 data-taking periods.}
\end{figure}
\clearpage
